# Supplementary material for: Achieving Scalable Capacity in Wireless Mesh Networks
Source: arXiv:2310.20227 source file (2023-10-31)
Supplement: Supplementary file 1 [file appendix.tex]

\appendix
\subsection{Derivation on (\ref{equ:I_re})}
\label{apx:equ:I_re}
Since the distance between a node in the $l$-th tier and the node in the center of the network is larger than or equal to $\left(\frac{3}{2}l\right) a$, it can be obtained that
\begin{equation*}
    \begin{aligned}
        I_j^{(r)} &\le \sum_{l=1}^{L_{r}} 6l \cdot CP \left(d_{l,min}^{(r)}\right)^{-\alpha} \\
        &= \sum_{l=1}^{L_{r}} 6l \cdot CP \left(\frac{3}{2}la\right)^{-\alpha} \\
        &=  \frac{6\cdot 2^{\alpha}C P}{\left(3a\right)^{\alpha}} \sum_{l=1}^{L_{r}}  \frac{1}{l^{\alpha-1}} \\
        &\le \frac{6\cdot 2^{\alpha}C P}{\left(3a\right)^{\alpha}} \left(1 + \int_{1}^{L_{r}}\frac{1}{l^{\alpha-1}} \mathrm{d}l \right) \\
        % &= \frac{6\cdot 2^{\alpha}C P}{\left(3a\right)^{\alpha}} \cdot \frac{\alpha-1-\frac{1}{L_{r}^{
        % \alpha-2}}}{\alpha - 2} \\
        &\le \frac{6\cdot 2^{\alpha}C P}{\left(3a\right)^{\alpha}} \cdot \frac{\alpha-1}{\alpha - 2} .
    \end{aligned}
\end{equation*}

\subsection{Derivation on (\ref{equ:I_perturb})}
\label{apx:equ:I_perturb}

Recall that the distance between a node in the $l$-th tier and the node in the center of the network is larger than or equal to $\left(\frac{3}{2}l-2\epsilon\right) a$, we can obtain that
\begin{equation*}
    \begin{aligned}
        I_j^{(p)} &\le \sum_{l=1}^{L} 6l \cdot CP \left(d_{l,min}^{(p)}\right)^{-\alpha} \\
        &= \sum_{l=1}^{L} 6l \cdot CP \left(\left(\frac{3}{2}l-2\epsilon\right) a\right)^{-\alpha} \\
        &=  \frac{6\cdot 2^{\alpha}C P}{a^{\alpha}} \sum_{l=1}^{L}  \frac{l}{\left(3l-4\epsilon \right)^{\alpha}} \\
        &\overset{(a)}{\le} \frac{6\cdot 2^{\alpha}C P}{a^{\alpha}} \left( \frac{1}{3-4\epsilon} + \sum_{l=2}^{L}  \frac{1}{\left(3l-4\epsilon \right)^{\alpha-1}} \right) \\
        &\le \frac{6\cdot 2^{\alpha}C P}{a^{\alpha}} \left( \frac{1}{3-4\epsilon} + \int_{l=1}^{L}  \frac{1}{\left(3l-4\epsilon \right)^{\alpha-1}} \mathrm{d}l \right) \\
        &= \frac{6\cdot 2^{\alpha}C P}{a^{\alpha}} \left( \frac{1}{3-4\epsilon} + \frac{\left(3-4\epsilon\right)^{2-\alpha}-\left(3L-4\epsilon\right)^{2-\alpha}}{\alpha-2} \right) \\
        &\le \frac{6\cdot 2^{\alpha}C P}{a^{\alpha}} \left( \frac{1}{3-4\epsilon} + \frac{1}{\left(\alpha-2\right)\left(3-4\epsilon\right)^{\alpha-2}} \right),
    \end{aligned}
\end{equation*}
where $(a)$ follows from the fact that $l < 3l-4\epsilon$ when $l \ge 2$ since $\epsilon < \frac{3}{4}$.

\subsection{Chernoff upper tail bound}
\label{apx:chernoff_upper_bound}
If $\xi$ is the sum of multiple independent indicator random variables, then
\begin{equation*}
    P[\xi \geq\left(1+\delta\right) E[\xi]] \leq \text{exp}\left(-\frac{\delta^{2} E[\xi]}{2+\delta}\right), \quad \delta>0.
\end{equation*}
